# Supplementary material for: HOH: Markerless Multimodal Human-Object-Human Handover Dataset with Large Object Count
Source: arXiv:2310.00723 source file (2024-05-03)
Supplement: Supplementary file 2 [file Paper_Forms_Template.pdf]

|    | giver id  | right/left     | mask?            | receiver id | right/left | mask?         |       |
|----|-----------|----------------|------------------|-------------|------------|---------------|-------|
|    | object id | giver response | receiver respons | gloved?     | bimanual?  | stopped here? | notes |
| 1  |           |                |                  |             |            |               |       |
| 2  |           |                |                  |             |            |               |       |
| 3  |           |                |                  |             |            |               |       |
| 4  |           |                |                  |             |            |               |       |
| 5  |           |                |                  |             |            |               |       |
| 6  |           |                |                  |             |            |               |       |
| 7  |           |                |                  |             |            |               |       |
| 8  |           |                |                  |             |            |               |       |
| 9  |           |                |                  |             |            |               |       |
| 10 |           |                |                  |             |            |               |       |
| 11 |           |                |                  |             |            |               |       |
| 12 |           |                |                  |             |            |               |       |
| 13 |           |                |                  |             |            |               |       |
| 14 |           |                |                  |             |            |               |       |
| 15 |           |                |                  |             |            |               |       |
| 16 |           |                |                  |             |            |               |       |
| 17 |           |                |                  |             |            |               |       |
| 18 |           |                |                  |             |            |               |       |
| 19 |           |                |                  |             |            |               |       |
| 20 |           |                |                  |             |            |               |       |
| 21 |           |                |                  |             |            |               |       |
| 22 |           |                |                  |             |            |               |       |
| 23 |           |                |                  |             |            |               |       |
| 24 |           |                |                  |             |            |               |       |
| 25 |           |                |                  |             |            |               |       |
| 26 |           |                |                  |             |            |               |       |
| 27 |           |                |                  |             |            |               |       |
| 28 |           |                |                  |             |            |               |       |
| 29 |           |                |                  |             |            |               |       |
| 30 |           |                |                  |             |            |               |       |

|    | giver id  | right/left     | mask?            | receiver id | right/left | mask?         |       |
|----|-----------|----------------|------------------|-------------|------------|---------------|-------|
|    | object id | giver response | receiver respons | gloved?     | bimanual?  | stopped here? | notes |
| 31 |           |                |                  |             |            |               |       |
| 32 |           |                |                  |             |            |               |       |
| 33 |           |                |                  |             |            |               |       |
| 34 |           |                |                  |             |            |               |       |
| 35 |           |                |                  |             |            |               |       |
| 36 |           |                |                  |             |            |               |       |
| 37 |           |                |                  |             |            |               |       |
| 38 |           |                |                  |             |            |               |       |
| 39 |           |                |                  |             |            |               |       |
| 40 |           |                |                  |             |            |               |       |
| 41 |           |                |                  |             |            |               |       |
| 42 |           |                |                  |             |            |               |       |
| 43 |           |                |                  |             |            |               |       |
| 44 |           |                |                  |             |            |               |       |
| 45 |           |                |                  |             |            |               |       |
| 46 |           |                |                  |             |            |               |       |
| 47 |           |                |                  |             |            |               |       |
| 48 |           |                |                  |             |            |               |       |
| 49 |           |                |                  |             |            |               |       |
| 50 |           |                |                  |             |            |               |       |
| 51 |           |                |                  |             |            |               |       |
| 52 |           |                |                  |             |            |               |       |
| 53 |           |                |                  |             |            |               |       |
| 54 |           |                |                  |             |            |               |       |
| 55 |           |                |                  |             |            |               |       |
| 56 |           |                |                  |             |            |               |       |
| 57 |           |                |                  |             |            |               |       |
| 58 |           |                |                  |             |            |               |       |
| 59 |           |                |                  |             |            |               |       |

|    | giver id  | right/left     | mask?            | receiver id | right/left | mask?         |       |
|----|-----------|----------------|------------------|-------------|------------|---------------|-------|
|    | object id | giver response | receiver respons | gloved?     | bimanual?  | stopped here? | notes |
| 60 |           |                |                  |             |            |               |       |
| 61 |           |                |                  |             |            |               |       |
| 62 |           |                |                  |             |            |               |       |
| 63 |           |                |                  |             |            |               |       |
| 64 |           |                |                  |             |            |               |       |
| 65 |           |                |                  |             |            |               |       |
| 66 |           |                |                  |             |            |               |       |
| 67 |           |                |                  |             |            |               |       |
| 68 |           |                |                  |             |            |               |       |
